# Supplementary material for: Leave-One-Out Neighborhood Smoothing for Graphons: Berry--Esseen Bounds and Edge-Wise Confidence Intervals
Source: arXiv:2602.02319 source file (2026-10-29)
Supplement: Supplementary file 1 [file additional_stress.tex]

\begin{table}[tb]
\centering
\caption{Additional stress-test results at $n=500$.
Point-estimation MSEs use $h_n=63$ and Gaussian inference uses $h_n=42$. The column $\widehat V/V$ reports a Monte Carlo mean.}
\label{tab:additional-stress-tests}
\small
\setlength{\tabcolsep}{4pt}
\begin{tabular}{lrrrrrr}
\toprule
Model & LOO MSE & ZLZ MSE & LOO cov. & ZLZ cov. & LOO width & $\widehat V/V$ \\
\midrule
Sinusoidal & 0.00377 & 0.00379 & 0.948 & 0.935 & 0.286 & 1.001 \\
Additive linear & 0.00463 & 0.00470 & 0.935 & 0.925 & 0.294 & 0.996 \\
Spiky & 0.00249 & 0.00252 & 0.921 & 0.925 & 0.237 & 0.978 \\
\bottomrule
\end{tabular}
\end{table}
